# Supplementary material for: Fine-Tuning and Prompt Engineering for Large Language Models-based Code Review Automation
Source: arXiv:2402.00905 source file (2024-06-17)
Supplement: Supplementary file 1 [file Appendix.tex]

\appendix

\begin{figure}[!h]
    \centering
    \begin{subfigure}{\columnwidth}
         \centering
         \includegraphics[width=\columnwidth, page = 3, trim = {0 3cm 0 0}, clip]{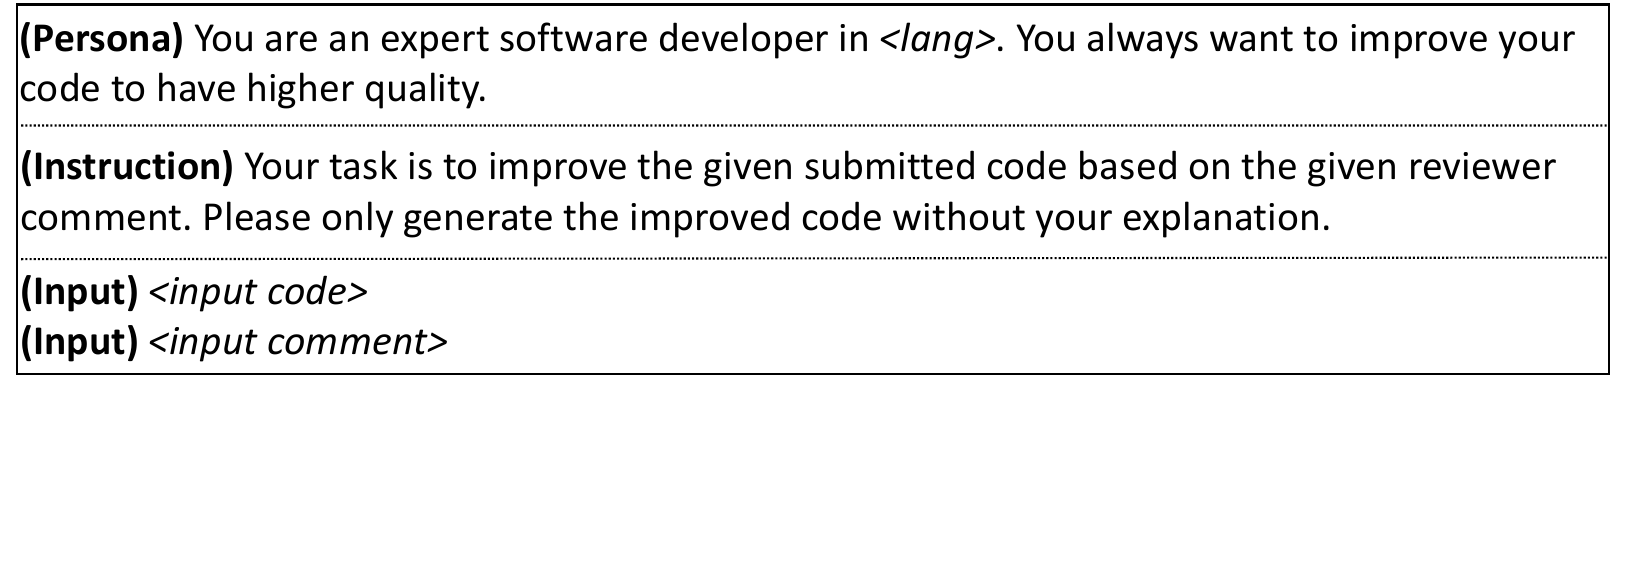}
         \caption{A prompt template for zero-shot learning (when a reviewer comment is available).}
         \label{fig:zero-shot prompt with comment new one 1}
     \end{subfigure}
    \par\bigskip
    \begin{subfigure}{\columnwidth}
         \centering
         \includegraphics[width=\columnwidth, page = 4, trim = {0 4cm 0 0}, clip]{figure/0-shot-prompt-templates_new.pdf}
         \caption{A prompt template for zero-shot learning (when a reviewer comment is not available).}
         \label{fig:zero-shot prompt without comment new one 1}
     \end{subfigure}
     \par\bigskip
     \begin{subfigure}{\columnwidth}
         \centering
         \includegraphics[width=\columnwidth, page = 3, trim = {0 3cm 0 0}, clip]{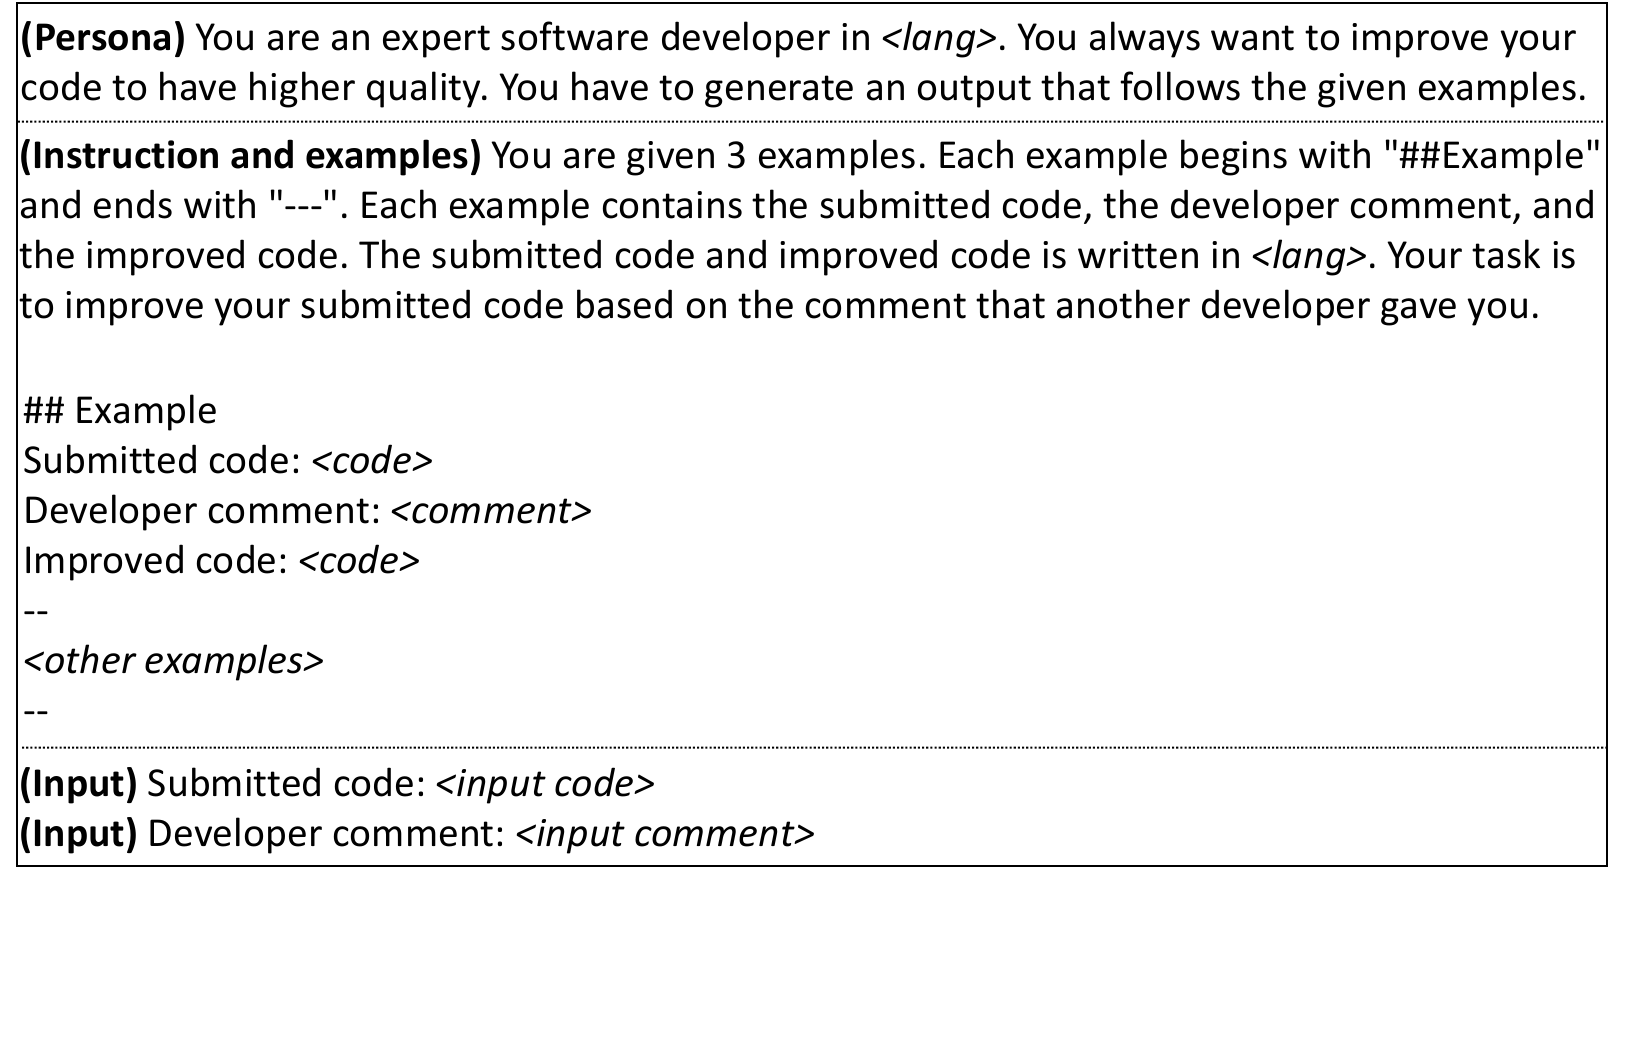}
         \caption{A prompt template for few-shot learning (when a reviewer comment is available).}
         \label{fig:few-shot prompt with comment new one 1}
     \end{subfigure}
     \par\bigskip 
     \begin{subfigure}{\columnwidth}
         \centering
         \includegraphics[width=\columnwidth, page = 4, trim = {0 4.5cm 0 0}, clip]{figure/few-shot-prompt-templates_new.pdf}
         \caption{A prompt template for few-shot learning (when a reviewer comment is not available).}
         \label{fig:few-shot prompt without comment new one 1}
     \end{subfigure}

    \caption{Prompt templates for performing zero-shot learning and few-shot learning with Magicoder \#1 (\textit{lang} refers to a programming language).}
    \label{fig:prompt-templates-new-one-1}
\end{figure}

\begin{figure}[!h]
    \centering
    \begin{subfigure}{\columnwidth}
         \centering
         \includegraphics[width=\columnwidth, page = 5, trim = {0 0 0 0}, clip]{figure/0-shot-prompt-templates_new.pdf}
         \caption{A prompt template for zero-shot learning (when a reviewer comment is available).}
         \label{fig:zero-shot prompt with comment new one 2}
     \end{subfigure}
    \par\bigskip
    \begin{subfigure}{\columnwidth}
         \centering
         \includegraphics[width=\columnwidth, page = 6, trim = {0 1cm 0 0}, clip]{figure/0-shot-prompt-templates_new.pdf}
         \caption{A prompt template for zero-shot learning (when a reviewer comment is not available).}
         \label{fig:zero-shot prompt without comment new one 2}
     \end{subfigure}
     \par\bigskip
     \begin{subfigure}{\columnwidth}
         \centering
         \includegraphics[width=\columnwidth, page = 5, trim = {0 0 0 0}, clip]{figure/few-shot-prompt-templates_new.pdf}
         \caption{A prompt template for few-shot learning (when a reviewer comment is available).}
         \label{fig:few-shot prompt with comment new one 2}
     \end{subfigure}
     \par\bigskip 
     \begin{subfigure}{\columnwidth}
         \centering
         \includegraphics[width=\columnwidth, page = 6, trim = {0 4cm 0 0}, clip]{figure/few-shot-prompt-templates_new.pdf}
         \caption{A prompt template for few-shot learning (when a reviewer comment is not available).}
         \label{fig:few-shot prompt without comment new one 2}
     \end{subfigure}

    \caption{Prompt templates for performing zero-shot learning and few-shot learning with Magicoder \#2 (\textit{lang} refers to a programming language).}
    \label{fig:prompt-templates-new-one-2}
\end{figure}

% Table generated by Excel2LaTeX from sheet 'results each RQ new format'
\begin{table*}[h]
  % \makegapedcells
  \centering
  \caption{The evaluation results of~\MagicoderZeroShot(persona is not included in input prompts).}
  \resizebox{\textwidth}{!}{
    \begin{tabular}{|l|c|c|c|c|c|c|c|c|c|c|c|c|}
    \hline
    \multicolumn{1}{|c|}{\multirow{2}[1]{*}{Approach}} & \multicolumn{2}{c|}{\CodeReviewerData} & \multicolumn{2}{c|}{\tufanoData (with comment)} & \multicolumn{2}{c|}{\tufanoData (without comment)} & \multicolumn{2}{c|}{Android} & \multicolumn{2}{c|}{Google} & \multicolumn{2}{c|}{Ovirt} \\
\cline{2-13}      & EM & CodeBLEU & EM & CodeBLEU & EM & CodeBLEU & EM & CodeBLEU & EM & CodeBLEU & EM & CodeBLEU \\
    \hline
    \MagicoderZeroShotPI & 9.92\% & 60.57\% & 6.12\% & 72.46\% & 2.39\% & 64.06\% & 0.00\% & 35.78\% & 0.00\% & 35.68\% & 0.00\% & 31.72\% \\
    \hline
    \MagicoderZeroShotPII & 11.80\% & 61.55\% & 6.65\% & 72.23\% & 1.33\% & 53.26\% & 0.31\% & 29.94\% & 0.00\% & 24.42\% & 0.00\% & 24.70\% \\
    \hline
    \end{tabular}%
  }
  \label{tab:magicoder-0-shot-no-persona}%
\end{table*}%

\begin{table*}[h]
  % \makegapedcells
  \centering
  \caption{The evaluation results of~\MagicoderZeroShot(persona is included in input prompts).}
  \resizebox{\textwidth}{!}{
    \begin{tabular}{|l|c|c|c|c|c|c|c|c|c|c|c|c|}
    \hline
    \multicolumn{1}{|c|}{\multirow{2}[1]{*}{Approach}} & \multicolumn{2}{c|}{\CodeReviewerData} & \multicolumn{2}{c|}{\tufanoData (with comment)} & \multicolumn{2}{c|}{\tufanoData (without comment)} & \multicolumn{2}{c|}{Android} & \multicolumn{2}{c|}{Google} & \multicolumn{2}{c|}{Ovirt} \\
\cline{2-13}      & EM & CodeBLEU & EM & CodeBLEU & EM & CodeBLEU & EM & CodeBLEU & EM & CodeBLEU & EM & CodeBLEU \\
    \hline
    \MagicoderZeroShotPI & 9.92\% & 59.48\% & 6.12\% & 72.57\% & 2.39\% & 56.29\% & 0.62\% & 36.81\% & 0.00\% & 35.93\% & 0.00\% & 31.10\% \\
    \hline
    \MagicoderZeroShotPII & 12.06\% & 61.54\% & 7.18\% & 70.56\% & 1.33\% & 37.57\% & 0.31\% & 27.21\% & 0.34\% & 25.35\% & 0.00\% & 24.34\% \\
    \hline
    \end{tabular}%
  }
  \label{tab:magicoder-0-shot-with-persona}%
\end{table*}%

\begin{table*}[!h]
  % \makegapedcells
  \centering
  \caption{The evaluation results of~\MagicoderFewShot(persona is not included in input prompts).}
  \resizebox{\textwidth}{!}{
    \begin{tabular}{|l|c|c|c|c|c|c|c|c|c|c|c|c|}
    \hline
    \multicolumn{1}{|c|}{\multirow{2}[1]{*}{Approach}} & \multicolumn{2}{c|}{\CodeReviewerData} & \multicolumn{2}{c|}{\tufanoData (with comment)} & \multicolumn{2}{c|}{\tufanoData (without comment)} & \multicolumn{2}{c|}{Android} & \multicolumn{2}{c|}{Google} & \multicolumn{2}{c|}{Ovirt} \\
\cline{2-13}      & EM & CodeBLEU & EM & CodeBLEU & EM & CodeBLEU & EM & CodeBLEU & EM & CodeBLEU & EM & CodeBLEU \\
    \hline
    \MagicoderFewShotPI & 19.84\% & 66.87\% & 5.85\% & 13.51\% & 3.20\% & 18.63\% & 0.31\% & 9.49\% & 1.02\% & 13.05\% & 0.89\% & 12.83\% \\
    \hline
    \MagicoderFewShotPII & 15.82\% & 60.56\% & 5.32\% & 14.04\% & 2.13\% & 15.80\% & 0.63\% & 7.31\% & 0.68\% & 9.53\% & 0.89\% & 8.09\% \\
    \hline
    \end{tabular}%
  }
  \label{tab:magicoder-few-shot-no-persona}%
\end{table*}%

\begin{table*}[!h]
  % \makegapedcells
  \centering
  \caption{The evaluation results of~\MagicoderFewShot(persona is included in input prompts).}
  \resizebox{\textwidth}{!}{
    \begin{tabular}{|l|c|c|c|c|c|c|c|c|c|c|c|c|}
    \hline
    \multicolumn{1}{|c|}{\multirow{2}[1]{*}{Approach}} & \multicolumn{2}{c|}{\CodeReviewerData} & \multicolumn{2}{c|}{\tufanoData (with comment)} & \multicolumn{2}{c|}{\tufanoData (without comment)} & \multicolumn{2}{c|}{Android} & \multicolumn{2}{c|}{Google} & \multicolumn{2}{c|}{Ovirt} \\
\cline{2-13}      & EM & CodeBLEU & EM & CodeBLEU & EM & CodeBLEU & EM & CodeBLEU & EM & CodeBLEU & EM & CodeBLEU \\
    \hline
    \MagicoderFewShotPI & 22.25\% & 67.32\% & 5.85\% & 11.82\% & 3.20\% & 17.45\% & 0.31\% & 9.72\% & 0.68\% & 14.17\% & 1.19\% & 14.23\% \\
    \hline
    \MagicoderFewShotPII & 13.67\% & 61.45\% & 5.32\% & 14.78\% & 1.60\% & 16.98\% & 0.63\% & 8.23\% & 0.68\% & 10.83\% & 0.59\% & 10.72\% \\
    \hline
    \end{tabular}%
  }
  \label{tab:magicoder-few-shot-with-persona}%
\end{table*}%

\section{More experiment results with Magicoder}

\kla{why do we need this? how is this appendix benefit the paper?}

In this section, we explain the experiment design for the experiments with Magicoder~\cite{wei2023magicoder} by using other prompts, and present the experiment results.

\textbf{Experiment design}:
To conduct the experiments, we first design prompt templates as shown in Figure~\ref{fig:prompt-templates-new-one-1} and Figure~\ref{fig:prompt-templates-new-one-2}.
Then, we perform zero-shot learning and few-shot learning with Magicoder~\cite{wei2023magicoder} by using the prompts in the aforementioned figures.
In the experiments, we obtain the samples from the testing set of each dataset with 95\% confidence level and 5\% confidence interval.

\textbf{Experiment result}:
Table~\ref{tab:magicoder-0-shot-no-persona} - Table~\ref{tab:magicoder-few-shot-with-persona} show the experiment results that we perform zero-shot learning and few-shot learning with Magicoder by using the prompts in Figure~\ref{fig:prompt-templates-new-one-1} and Figure~\ref{fig:prompt-templates-new-one-2}.
In the tables, \MagicoderZeroShotPI~and \MagicoderZeroShotPII~denote Magicoder that is performed zero-shot learning by using the prompts in Figure~\ref{fig:prompt-templates-new-one-1} and Figure~\ref{fig:prompt-templates-new-one-2}, respectively.
Similarly, \MagicoderFewShotPI~and \MagicoderFewShotPII~ denote Magicoder that is performed few-shot learning by using the prompts in Figure~\ref{fig:prompt-templates-new-one-1} and Figure~\ref{fig:prompt-templates-new-one-2}, respectively.
We explain the experiment results below.

Table~\ref{tab:magicoder-0-shot-no-persona} shows that when persona is not included in input prompts, \MagicoderZeroShotPII~achieves at least 8.66\% higher EM than \MagicoderZeroShotPI~(except for the Tu\-fano\textsubscript{data}(without comment) while \MagicoderZeroShotPI~ac\-hieves at least 0.32\% higher CodeBLEU than \MagicoderZeroShotPII.
Similarly, Table~\ref{tab:magicoder-0-shot-with-persona} shows that when persona is included in input prompts, \MagicoderZeroShotPII~achieves at least 17.32\% higher EM than \MagicoderZeroShotPI~(except for the Tu\-fano\textsubscript{data}(without comment) while \MagicoderZeroShotPI~achieves at least 2.85\% higher CodeBLEU than \MagicoderZeroShotPII.

% Table~\ref{tab:magicoder-0-shot-with-persona} shows that 

Table~\ref{tab:magicoder-few-shot-no-persona} shows that when persona is not included in input prompts, \MagicoderFewShotPI~achieves at least 9.96\% higher EM and 10.42\% higher CodeBLEU than \MagicoderFewShotPII.
Similarly, when persona is included in input prompts, \MagicoderFewShotPI~achieves at least 9.96\% higher EM and 2.77\% higher CodeBLEU than Magi\-coder-P2\textsubscript{Few-shot}.

% Table~\ref{tab:magicoder-few-shot-with-persona} shows that 

The results indicate that when zero-shot learning is performed with Magicoder by using different prompts, Magi\-coder-P2\textsubscript{Few-shot} can correctly generate more improved code than \MagicoderZeroShotPI, but \MagicoderZeroShotPI~can generate improved code more similar to the actual improved code than \MagicoderZeroShotPII.
In contrast, when few-shot learning is performed with Magicoder by using different prompts, \MagicoderZeroShotPI~can correctly generate more improved code and generate improved code more similar to the actual improved code than \MagicoderZeroShotPII.
